# Supplementary material for: Magnetically driven short-range order can explain anomalous measurements in CrCoNi
Source: arXiv:2004.09086 ancillary file (2021-03-31)
Supplement: Supplementary file 1 [file SI_Appendix.pdf]

# Supplementary Information for

## Magnetically driven short-range order can explain anomalous measurements in CrCoNi

**Flynn Walsh, Mark Asta, Robert O. Ritchie**

**Robert O. Ritchie.**
**E-mail:roritchie@lbl.gov**

### This PDF file includes:

Supplementary text
Figs. S1 to S3 (not allowed for Brief Reports)
SI References

## Supporting Information Text

**Discussion of simulation methodology.** It should be noted that predicting finite temperature SRO using 0-K spin-polarized DFT involves some level of approximation. Namely, while long-range magnetic order may not persist at the temperatures of chemical SRO formation, the local magnetic interactions responsible for DFT energies (see Fig. S1) are expected to still drive chemical rearrangement via magnetic SRO, which has been predicted to exist in transition metals at a length scale on the order of our supercell size (1–3). We also assume that a system's magnetic structure readily adapts to chemical changes and a 0-K calculation accurately represents a finite temperature snapshot. Furthermore, our calculations do not account for the possibility of spin fluctuations as are seen in elemental Ni and have been predicted in some similar materials (4).

Another concern is that noncollinear arrangements of moments could offer a pathway to resolving magnetic frustration, but this behavior is rarely observed in Cr clusters (5) and, consistent with Ref. (6), only collinear states could be converged. Although this may not disprove the possibility of a noncollinear solution, a complete absence of noncollinearity in the relaxation of randomly initialized moments suggests it is unlikely. Indeed, a configuration's final magnetic structure appeared independent of initial local moments, although simulation times varied significantly. After extensive testing, moments were generally initialized to -2 $\mu_B$/atom for Cr and 1 $\mu_B$/atom for Ni and Co to optimize convergence speed. In general, no appreciable difference in results was found between the chosen simulation parameters, which follow Ref. (7), and those reported by Ref. (8) or (9).

One possible counterargument to the existence of spin-ordered SRO is that the increase in total volume seen in Fig. 5(a) contradicts the X-ray diffraction measurements of Ref. (10), which show a slightly reduced lattice constant in aged samples. However, the volume difference between experiment and any DFT calculation dwarfs the variation among individual ordering models, presumably in part due to thermal expansion. Given their significantly stronger magnetic couplings, the SRO states could reasonably exhibit reduced thermal expansion and lower room temperature volume despite slightly larger ground state structures.

## References


1. H. Capellmann, V. Viera, Strong short range magnetic order in ferromagnetic transition metals above $T_c$: A theoretical explanation. *Solid State Commun.* **43**, 747–750 (1982).
2. V. Heine, A. I. Liechtenstein, O. N. Mryasov, On the Origin of Short-Range Order above $T_c$ in Fe, Co, Ni. *Europhys. Lett. (EPL)* **12**, 545–550 (1990).
3. N. B. Melnikov, B. I. Reser, G. V. Paradezhenko, Short-range order in metals above the Curie temperature. *AIP Adv.* **8**, 101402 (2018).
4. B. Schönfeld, et al., Local order in Cr-Fe-Co-Ni: Experiment and electronic structure calculations. *Phys. Rev. B* **99**, 014206 (2019).
5. P. Ruiz-Díaz, J. L. Ricardo-Chávez, J. Dorantes-Dávila, G. M. Pastor, Magnetism of small Cr clusters: Interplay between structure, magnetic order, and electron correlations. *Phys. Rev. B* **81**, 224431 (2010).
6. C. Niu, C. R. LaRosa, J. Miao, M. J. Mills, M. Ghazisaeidi, Magnetically-driven phase transformation strengthening in high entropy alloys. *Nat. Commun.* **9**, 1363 (2018).
7. J. Ding, Q. Yu, M. Asta, R. O. Ritchie, Tunable stacking fault energies by tailoring local chemical order in CrCoNi medium-entropy alloys. *Proc. National Acad. Sci.* **115**, 8919–8924 (2018).
8. A. Tamm, A. Aabloo, M. Klintenberg, M. Stocks, A. Caro, Atomic-scale properties of Ni-based FCC ternary, and quaternary alloys. *Acta Materialia* **99**, 307–312 (2015).
9. B. Yin, S. Yoshida, N. Tsuji, W. A. Curtin, Yield strength and misfit volumes of NiCoCr and implications for short-range-order. *Nat. Commun.* **11**, 2507 (2020).
10. R. Zhang, et al., Short-range order and its impact on the CrCoNi medium-entropy alloy. *Nature* **581**, 283–287 (2020).

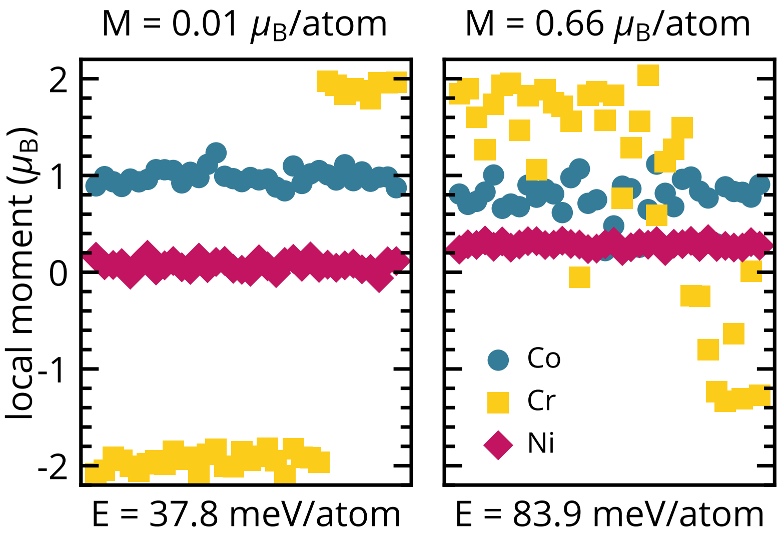


**Fig. S1.** Local atomic moments, colored by element, calculated for a spin-ordered configuration under two different magnetic states. On the left, moments are fully relaxed, leading to approximately 0 $\mu_B$ Ni moments, 1 $\mu_B$ Co moments, and $\pm 2$ $\mu_B$ Cr moments. Naively, flipping this cell's Cr spins would produce a $\sim \frac{2}{3}$ $\mu_B$/atom net magnetization, although controlling individual moments is computationally challenging. For the right plot, the constraint of $\frac{2}{3}$ $\mu_B$/atom total moment is imposed on the simulation cell. Most Cr spins flip to satisfy the constraint, with a much smaller effect on Ni and Co moments; the persistence of up and down Cr and change in many moment magnitudes demonstrates the strength of the system's magnetic interactions. The ferromagnetic state (right) is 46 meV/atom higher in energy than the magnetically relaxed state (left), which is very close to the average gap between quasirandom and spin-ordered configurations (49 meV/atom). This demonstrates how the spin-ordered model's favorability originates from its magnetic interactions and not simply the associated chemical rearrangement.

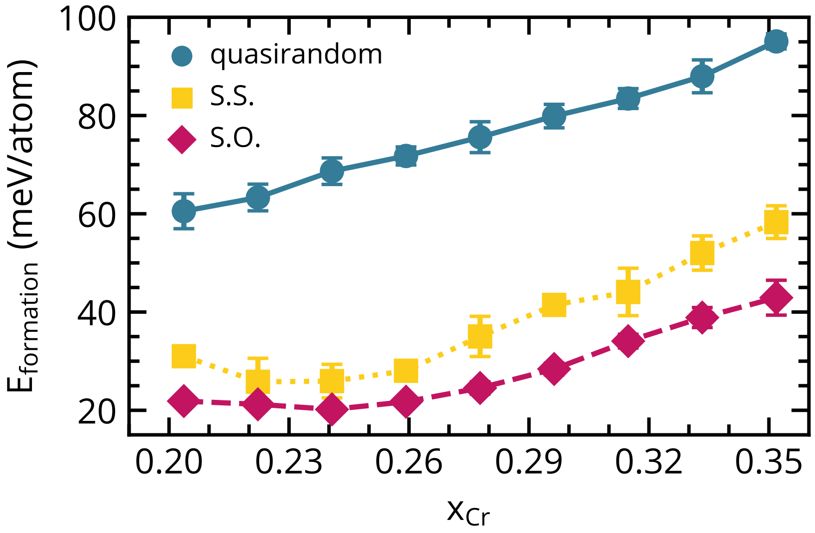


**Fig. S2.** An analog of Fig. 4, with DFT formation energy in place of magnetization. Below $x_{\mathrm{Cr}} \approx 0.28$, the energy difference between simple structural ("S.S.") and spin-ordered ("S.O.") configurations is notably reduced. In this region, predictions made using the spin-ordered model diverge from experimental data. These observations suggest that the realized ordering state may change with composition.

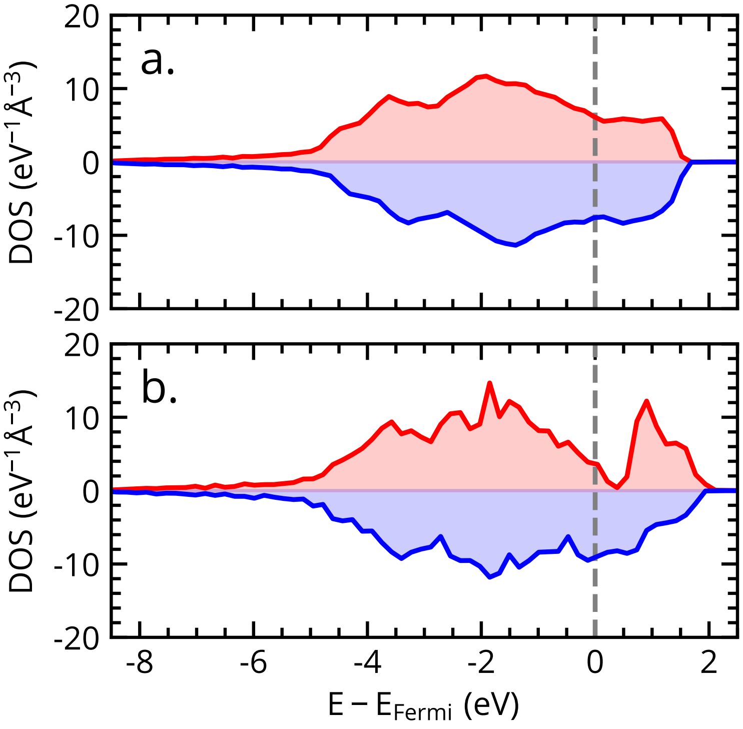


**Fig. S3.** Total spin-polarized density of states for configurations representing (a) quasirandom and (b) spin-ordered CrCoNi. The dashed line indicates the Fermi level. Calculations used were performed using a $6 \times 6 \times 6$ Monkhorst-Pack grid.
